# Supplementary material for: Breaking the Limits of Message Passing Graph Neural Networks
Source: arXiv:2106.04319 source file (2021-06-08)
Supplement: Supplementary file 1 [file appendixWL.tex]

The universality of a GNN is based on its ability to embed two non-isomorphic graphs to distinct points in the target feature space. A model which can distinguish all pairs of non-isomorphic graphs is a universal approximator. Since it is not known if the graph isomorphism problem can be solved in polynomial time or not, this problem is neither NP-complete nor P, but NP-intermediate \cite{takapoui2016linear}. One of the oldest but prominent polynomial approach is the Weisfeiler-Lehman Test (abbreviated WL-test) which gives 
%named WL test gives
sufficient but not enough evidence. WL test can be extended by taking into account higher order of node tuple within the iterative process. These extensions are denoted as $k$-WL test, where $k$ is equals to the order of the tuple. It is important to mention that an higher order of tuple leads to a better ability to distinguish two non-isomorphic graphs (with the exception for $k=2$) ~\cite{arvind2020weisfeiler}.

%enumerated by the order of node tuple used in the iteration such as 1-WL, 2-WL,..,k-WL where the one is more powerful than its ancestor in terms of ability to distinguish two non-isomorphic graphs \cite{arvind2020weisfeiler}.

The 1-WL test, known as vertex coloring, starts with the given initial color of nodes if available (unless assume all nodes are monochromatic, so all nodes color is the same, $H_v^{(0)}=1$) and updates the color by the following iteration:
\begin{equation}
  \label{eq:wl1}
  H_v^{(t+1)} =\sigma \left( H_v^{(t)}~ |\left\{ H_u^{(t)} : u \in \mathcal{N}(v) \right\} \right),
\end{equation}
where $H_v^{(t)}$ is the color of vertex $v$ at iteration $t$, $\mathcal{N}(v)$ is the set of neighbours of vertex $v$, the concatenation operator is represented by $|$ and order invariant set can be shown by $\{.\}$, which is % where we
generally implemented %it
by stacking all colors in the set and sorting them alphabetically. To avoid the new color of vertex become bigger after each iteration, $\sigma(.)$ function performs the recoloring step where it assigns a new color identifier to the every new created unique color. The test should be done in parallel for two graphs and iterative process is stopped when the histograms are not changing between two iterations.
%of color is not changing between two iterations. and color histograms are compared after each iteration.
% after every iteration histogram of vertex color should be compared.
If the histograms are different in any iteration we can conclude that the graphs are not isomorphic. Conversely, two same histograms may be computed even for non-isomorphic graphs.
%Even after new iteration, the colors of the nodes do not change and still the histograms are the same, we can end the iteration however cannot be sure that these two graphs are not isomorphic. 

Higher order WL tests use the same algorithm while their color update schema is slightly different. 2-WL test uses second order tuple of nodes (all ordered pairs of nodes), thus it needs $\mathbf{H} \in \mathbb{R}^{n \times n}$ matrix, where initial colors have two more colors than initial vertex colors as defined by:
\begin{equation}
  \label{wl2initial}
  \mathbf{H}_{v,u}^{(0)} = \left\{
        \begin{array}{l@{\text{ ~~~~if~ }}l}
            H_v^{(0)} & v = u \\           
            edge & u \in \mathcal{N}(v) \\  
            nonedge & u \not\in \mathcal{N}(v) \\
        \end{array}
    \right. 
\end{equation}
Then the iteration uses following schema where $[n]$ is the set of node identifiers.
\begin{equation}
  \label{eq:wl2}
  \mathbf{H}_{v,u}^{(t+1)} =\sigma \left( \mathbf{H}_{v,u}^{(t)}~ |\left\{ \mathbf{H}_{v,k}^{(t)} : k \in [n] \right\} |\left\{ \mathbf{H}_{k,u}^{(t)} : k \in [n] \right\} \right),
\end{equation}
Although for $k\geq2$, $(k+1)$-WL $>$ $(k)$-WL, it is not true for $k=1$, thus given 2-WL in Eq.\ref{eq:wl2} is no more powerful than 1-WL in \ref{eq:wl1} \cite{maron2019provably}. To clarify this point,
Folkore WL (FWL) test is defined such as 1-WL=1-FWL, but for $k \geq 2$, we have $(k+1)$-WL $\approx$ $(k)$-FWL~\cite{maron2019provably}.
%In this point, there is another version of WL named Folklore WL (FWL) which is exactly the same for $k=1$, thus 1-WL=1-FWL but for $k\geq2$, $(k+1)$-WL $\approx$ $(k)$-FWL \cite{maron2019provably}.
The iteration process of 2-FWL can be shown by following equation;
\begin{equation}
  \label{eq:fwl2}
  \mathbf{H}_{v,u}^{(t+1)} =\sigma \left( \mathbf{H}_{v,u}^{(t)}~ |\left\{ \left( \mathbf{H}_{v,k}^{(t)} | \mathbf{H}_{k,u}^{(t)} \right) : k \in [n]  \right\} \right),
\end{equation}

In literature, there is a conflict to use the order of the WL test. Some papers use defined WL test order in Eq.~\ref{eq:wl1} and Eq.~\ref{eq:wl2} \cite{123lehmango, maron2019provably} but some others use FWL order under the name of WL such as in \cite{abboud2020surprising,arvind2020weisfeiler,takapoui2016linear}. In this paper, we explicitly mention both WL and FWL equivalent such as 3-WL (or 2-FWL) to alleviate ambiguities.
